# Supplementary material for: Publicly available datasets of breast histopathology H&E whole-slide images: A scoping review
Source: arXiv:2306.01546 source file (2023-12-06)
Supplement: Supplementary file 2 [file Supplementary_material_2.pdf]

## (a) Detail of search queries used in literature databases

| # | Database | Search details | Filter | Date | Results |
|---|---|---|---|---|---|
| 1 | PubMed | Via Oria.no electronic Library :<br>All fields contain (“deep learning” OR “machine learning”) AND all fields contain (“whole slide images” OR “WSI”) AND all fields contain (breast) AND All fields contain (histology OR histopathology OR pathology) AND All fields contain (data OR dataset OR “data set”) | 2015- 2023<br>Full text<br>English | 07/06/2023 | 524 |
| 2 | ACM | [[All: "deep learning"] OR [All: "machine learning"]] AND [[All: "whole slide images"] OR [All: "wsi"]] AND [All: breast] AND [[All: histology] OR [All: histopathology] OR [All: pathology]] AND [[All: data] OR [All: dataset] OR [All: "data set"]] | [E-Publication Date: (01/01/2015 TO 07/06/2023)] | 07/06/2023 | 48 |
| 3 | Web of Science | Via Oria.no electronic Library :<br>(“deep learning” OR “machine learning”) AND (“whole slide images” OR “WSI”) AND (breast) AND (histology OR histopathology OR pathology) AND (data OR dataset OR “data set”) | 2015- 2023<br>Full text<br>English | 07/06/2023 | 120 |
| 4 | Science direct | Via Oria.no electronic Library :<br>(“deep learning” OR “machine learning”) AND (“whole slide images” OR “WSI”) AND (breast) AND (histology OR histopathology OR pathology) AND (data OR dataset OR “data set”) | 2015- 2023<br>Full text<br>English | 07/06/2023 | 116 |
| 5 | Medline via Ovid | All fields contain (“deep learning” OR “machine learning”) AND all fields contain (“whole slide images” OR “WSI”) AND all fields contain (breast) AND All fields contain (histology OR histopathology OR pathology) AND All fields contain (data OR dataset OR “data set”) | 2015- 2022<br>English | 07/06/2023 | 329 |
| 6 | Semantic scholar | Via Oria.no electronic Library :<br>(“deep learning” OR “machine learning”) AND (“whole slide images” OR “WSI”) AND (breast) AND (histology OR histopathology OR pathology) AND (data OR dataset OR “data set”) | 2015- 2023<br>Full text<br>English | 07/06/2023 | 174 |
| 7 | IEEE-explore | In all metadata (“deep learning” OR “machine learning”) AND in all metadata (“whole slide images” OR “WSI”) AND in all metadata (breast) AND in all metadata (histology OR histopathology OR pathology) AND in all metadata (data OR dataset OR “data set”) | 2015- 2022 | 07/06/2023 | 19 |
| 8 | MDPI | Via Oria.no electronic Library :<br>All fields (“deep learning” OR “machine learning”) AND all fields (“whole slide images” OR “WSI”) AND all fields (breast) AND All fields (histology OR histopathology OR pathology) AND All fields(data OR dataset OR “data set”) | 2015- 2023<br>Full text<br>English | 07/06/2023 | 223 |
| 9 | dbpl | Breast wsi | | 07/06/2023 | 3 |

### (b) Search queries used in medical image databases, research data repositories, and challenges

| # | Source | Link | Search queries used | Date | Results |
|---|---|---|---|---|---|
| 1 | The Cancer Imaging Archive (TCIA) | https://www.cancerimagingarchive.net/histopathology-imaging-on-tcia/ | Breast<br>brca | 07/06/2023 | CPTAC-BRCA<br>Post-Nat-BRCA<br>SLN-Breast |
| 2 | National Cancer Institute – GDC Data Portal (NIH) | https://portal.gdc.cancer.gov/projects/TCGA-BRCA | Breast<br>brca | 07/06/2023 | TCGA-BRCA |
| 3 | Grand Challenge | https://grand-challenge.org/challenges/ | Breast histology<br>breast pathology<br>breast whole slide image<br>breast wsi | 07/06/2023 | ICIAR-2018<br>HEROHE<br>Camelyon 16<br>Camelyon 17<br>ACROBAT<br>BCNB<br>TIGER |
| 4 | Figshare | https://figshare.com/ | (“whole slide images” OR “WSI”) AND (breast) AND (histology OR histopathology OR pathology) AND (data OR dataset OR “data set”) | 07/06/2023 | No WSI dataset of breast |
| 5 | Zenodo | https://zenodo.org/ | Breast histology<br>breast pathology<br>breast whole slide image<br>breast wsi<br><br>Filter: datasets | 07/06/2023 | BACH<br>subsets of DRYAD, TCGA-BRCA, Camelyon 16 |
| 6 | Google data research | https://datasetsearch.research.google.com/ | (“whole slide images” OR “WSI”) AND (breast) AND (histology OR histopathology OR pathology) | 07/06/2023 | BACH<br>DRYAD<br>Camelyon 16<br>Camelyon 17<br>Subset of TCGA-BRCA |
| 7 | Papers with code | https://paperswithcode.com/datasets | Breast histology<br>breast pathology<br>breast whole slide image<br>breast wsi | 07/06/2023 | BRACS |
| 8 | Kaggle | https://www.kaggle.com/datasets | Breast histology<br>breast pathology<br>breast whole slide image<br>breast wsi | 07/06/2023 | BACH |
| 9 | Github | https://github.com/ | Breast histology<br>breast pathology<br>breast whole slide image<br>breast wsi | 07/06/2023 | No WSI dataset of breast |
