# Supplementary material for: Publicly available datasets of breast histopathology H&E whole-slide images: A scoping review
Source: arXiv:2306.01546 source file (2023-12-06)
Supplement: Supplementary file 3 [file Supplementary_material_3.pdf]

**List of breast H&E image tiles (patches) datasets**

| Name | Parent data | URL (repository or paper) |
|---|---|---|
| AMIDA 2013 (MICCAI 2013) | - | https://doi.org/10.1016/j.media.2014.11.010 |
| Breast Cancer Immunohistochemical Image (BCI) | - | https://bupt-ai-cz.github.io/BCI/ |
| BACH (ICIAR 2018) | - | https://iciar2018-challenge.grand-challenge.org/ |
| Breast Cancer Semantic Segmentation (BCSS) | TCGA | https://github.com/PathologyDataScience/BCSS |
| BioImaging 2015 (BICBH) | - | https://doi.org/10.3390/cancers13236116 |
| BisQue | - | https://doi.org/10.1016/j.jmir.2019.11.001 |
| BNS | - | https://doi.org/10.1186/s42490-019-0026-8 |
| Breast Histopathology images (BHI) | - | https://doi.org/10.1007/s11042-021-11775-2 |
| Breast PathQ (SPIE) | - | https://breastpathq.grand-challenge.org/ |
| Breast Cancer Histopathological Database (BreakHis) | - | https://web.inf.ufpr.br/vri/databases/breast-cancer-histopathological-database-breakhis/ |
| Breast Histopathology Images (IDC) | - | https://www.kaggle.com/datasets/paultimothymooney/breast-histopathology-images |
| BreCaHAD | - | https://doi.org/10.1186\%2Fs13104-019-4121-7 |
| Burnasyan (Federal Medical Biophysical Center) | - | https://github.com/aborbat/burnasyan_br |
| Databiox | - | https://databiox.com/ |
| Data science bowl 2018 | - | https://doi.org/10.1109/ICCIT-144147971.2020.9213817 |
| ERBCa+ | - | https://doi.org/10.1007/978-3-030-00949-6_18 |
| Histobreast | - | https://doi.org/10.1038/s41597-020-0500-0 |
| Janowczyk Nuclei segmentation dataset | TCGA | http://www.andrewjanowczyk.com/use-case-1-nuclei-segmentation/ |
| Kumar | TCGA | https://paperswithcode.com/dataset/kumar |
| MITOS(ICPR2012) | - | http://ludo17.free.fr/mitos_2012/index.html |
| Mitos \Atypia 14 (ICPR2014) | - | https://mitos-atypia-14.grand-challenge.org/ |
| KIMIA path24 | - | https://doi.org/10.1016/j.artmed.2019.101743 |
| KIMIA path 960 | - | https://www.kaggle.com/datasets/ambarish/kimia-path-960 |

| | | |
|---|---|---|
| METABRIC | - | https://doi.org/10.1016/j.asoc.2020.106238 |
| MICCAI 2018 (MoNuSeg) | TCGA | https://monuseg.grand-challenge.org/ |
| MItosis Domain Generalization (MICCAI-MIDOG challenge 2021) | - | https://midog2021.grand-challenge.org/ |
| Data from Ohio State University Cancer Institutional | - | https://zenodo.org/record/7514392 |
| PatchCamelyon | Camelyon | https://patchcamelyon.grand-challenge.org/ |
| SCAN algorithm dataset | - | https://data.mendeley.com/datasets/sc878z8pm3/1 |
| TNBC Nuclei Segmentation | - | https://github.com/PeterJackNaylor/DRFNS |
| Tata Medical Center (TMC) | - | https://doi.org/10.1007/s00138-020-01122-0 |
| UCSB (BCC) | - | https://doi.org/10.1145/3093293.3093307 |
