# Supplementary material for: Publicly available datasets of breast histopathology H&E whole-slide images: A scoping review
Source: arXiv:2306.01546 source file (2023-12-06)
Supplement: Supplementary file 4 [file Supplementary_material_4.pdf]

**List of private datasets of breast H\&E whole slide images**

| Dataset name | Study | Available upon agreement |
|---|---|---|
| ABCTB | https://doi.org/10.3390/diagnostics11081406 | YES |
| ABiM | https://doi.org/10.1158/0008-5472.CAN-21-0482 | NO |
| ACCC | https://doi.org/10.3390/cancers12123687 | NO |
| AIDPATH | https://doi.org/10.3390/app10217761 | NO |
| Bpath | https://doi.org/10.1111/his.13035 | NO |
| BRCA-08 | https://doi.org/10.1016/j.media.2020.101788 | NO |
| CBCS | https://doi.org/10.1038\%2Fs41523-018-0079-1 | YES |
| ClinSeq-BC | https://doi.org/10.1158/0008-5472.CAN-21-0482<br>https://doi.org/10.1016/j.annonc.2021.09.007 | NO |
| DROID | https://doi.org/10.1007/s10278-020-00384-4 | YES |
| DUKE | https://doi.org/10.1038/s41523-020-00205-5 | YES |
| GTEx | https://doi.org/10.1371/journal.pcbi.1006269 | YES |
| Hakuaikai Sagara Hospital | https://doi.org/10.1007/s10549-019-05390-x | YES |
| Herlev and Gentofte Hospital | https://doi.org/10.3390/cancers13123050 | NO |
| Rabat Histopathology department of the NIO | https://doi.org/10.1186/s13104-022-05936-1 | YES |
| Mayo Clinic, Rochester | https://doi.org/10.1038/s41523-021-00378-7 | YES |
| Memorial Sloan Kettering Cancer Center | https://doi.org/10.1038/s41379-021-00807-9 | YES |
| METABRIC | https://doi.org/10.3390/diagnostics11081406 | YES |
| NCI PDMR | https://doi.org/10.1145/3311790.3396663 | YES |
| PathLake | https://doi.org/10.1016/j.ajpath.2021.02.024 | NO |
| PathoEMR | https://doi.org/10.1186/s12911-020-01340-6 | NO |
| Pathology registries in Vermont and New Hampshire | https://doi.org/10.1007/s10278-016-9873-1 | NO |

| | | |
|---|---|---|
| Private data collected in 5 centers from Netherlands and Germany | https://doi.org/10.7717/peerj.8242 | NO |
| Samsung Medical Center (SMC) | https://doi.org/10.1186/s13000-020-00995-z | YES |
| SCAN-B study | https://doi.org/10.1016/j.annonc.2021.09.007 | NO |
| SöS-BC-1 | https://doi.org/10.1016/j.annonc.2021.09.007 | NO |
| St. George Breast Boost study | https://doi.org/10.3390\%2Fcancers12092365 | YES |
| SYSUCC | https://doi.org/10.1016/j.ebiom.2021.103492 | YES |
| Tissue slide database of Motic Corporation | https://doi.org/10.1016/j.cmpb.2018.02.020 | NO |
| University of Pittsburgh Medical Center (UPMC) | https://doi.org/10.1016/j.media.2020.101757<br>https://doi.org/10.1186/s13000-020-00995-z<br>https://doi.org/10.5858/arpa.2020-0034-OA | YES |
| University of Wisconsin at Madison | https://doi.org/10.1016/j.media.2020.101938 | YES |
| West China Hospital | https://doi.org/10.1186/s12967-021-03020-z | YES |
| Dataset from Semmelweis University | https://doi.org/10.3390/diagnostics12092161 | NO |
| Private clinical dataset from China | https://doi.org/10.1155/2022/2961610 | YES |
| UNC CBCS | https://doi.org/10.3390%2Fcancers14092148 | NO |
| AIDA BRLN | https://doi.org/10.3390%2Fcancers14215424 | YES |
| Dataset from Institut Curie | https://doi.org/10.1016%2Fj.xcrm.2022.100872 | NO |
| Dataset from Cancer Hospital, Chinese Academy of Medical Sciences | https://doi.org/10.1016/j.compbiomed.2022.105569 | NO |
| Nottingham University Hospital dataset | https://doi.org/10.1016/j.media.2022.102486 | NO |
| Komen Tissue Bank | https://doi.org/10.1186%2Fs13058-022-01541-z | YES |
| SingHealth data from Singapore | https://doi.org/10.1038/s41374-021-00689-0 | YES |
| University Medical Centre Utrecht | https://doi.org/10.1136%2Fbmjopen-2022-067437 | NO |
| caMicroscope digital platform | https://doi.org/10.3390/cancers14102467 | NO |

| | | |
|---|---|---|
| Data from Yamaguchi University, Tokyo Medical University, and Weill Cornell Medicine | https://doi.org/10.1002%2Fcjp2.314 | YES |
| BCMT from Xiangya Hospital | https://doi.org/10.3389%2Ffonc.2022.858453 | NO |
| Dataset from one hospital, China | https://doi.org/10.1145/3562007.3562048 | YES |
| Dataset from Emory Decatur Hospital | https://doi.org/10.1016%2Fj.jpi.2023.100311 | NO |
| Black Women's Health Study | https://doi.org/10.1186%2Fs13058-022-01577-1 | YES |
| Dataset from Yale School of Medicine | https://doi.org/10.1038%2Fs41379-021-00911-w | YES |
| Fudan University Shanghai Cancer Center | https://doi.org/10.21037%2Fjtd-23-445 | YES |
| Dataset from Ohio State University | https://doi.org/10.3389/fmed.2022.886763 | YES |
| NHS and NHSII cohorts from US | https://doi.org/10.1186%2Fs13058-023-01638-z | YES |
| ECOG and TMC datasets from US | https://doi.org/10.1038%2Fs41523-023-00545-y | YES |
| Dataset from Ajou University Medical Center in Republic of Korea | https://doi.org/10.3390%2Fdiagnostics12102340 | YES |
| Dataset from Southwestern Medical University Hospital | https://doi.org/10.1186%2Fs12885-023-10817-2 | YES |
| Dataset from Mount Sinai Health Care System | https://doi.org/10.1186%2Fs13058-022-01592-2 | YES |
| National Taiwan University Hospital | https://doi.org/10.3390%2Fdiagnostics12040990 | YES |
| International University of Health and Welfare (IUHW), Mita Hospital (Tokyo, Japan) and Kamachi Group Hospitals (total four hospitals: Wajiro, Shinkuki, Shinkomonji, and Shinmizumaki Hospital) (Fukuoka, Japan) | https://doi.org/10.1371%2Fjournal.pone.0275378 | YES |

* Not all of the listed private datasets are used in the included papers.
