# Supplementary material for: Publicly available datasets of breast histopathology H&E whole-slide images: A scoping review
Source: arXiv:2306.01546 source file (2023-12-06)
Supplement: Supplementary file 5 [file Supplementary_material_5.pdf]

## Supplement 5: Available clinical variables for breast H&E WSI datasets

The following tables present the available clinical variables in the six datasets checkmarked in Table 1 of the manuscript.

*Table 1. TCGA-BRCA dataset*

| | Variable | Description |
|---|---|---|
| 1 | Diagnosis Age | Range= [26, 90], Median=58 |
| 2 | Neoplasm Disease Stage American Joint Committee on Cancer Code | categories: NA, STAGE I, STAGE IA, STAGE IB, STAGE II, STAGE IIA, STAGE IIB, STAGE III, STAGE IIIA, STAGE IIIB, STAGE IIIC, STAGE IV, STAGE X |
| 3 | American Joint Committee on Cancer Publication Version Type | categories: NA, 6th, 7th |
| 4 | Aneuploidy Score | Range= [0, 35], Median=11 |
| 5 | Buffa Hypoxia Score | Range= [-49, 47], Median=-13 |
| 6 | Cancer Type | Breast cancer |
| 7 | TCGA PanCanAtlas Cancer Type Acronym | BRCA |
| 8 | Cancer Type Detailed | categories: Breast Invasive Lobular Carcinoma, Breast Invasive Ductal Carcinoma, Breast Invasive Carcinoma (NOS), Breast Invasive Mixed Mucinous Carcinoma, Metaplastic Breast Cancer, Invasive Breast Carcinoma |
| 9 | Last Communication Contact from Initial Pathologic Diagnosis Date | Range= [-31, 8605], Median=757 |
| 10 | Birth from Initial Pathologic Diagnosis Date | Range= [-32873, -9706], Median=-21534 |
| 11 | Last Alive Less Initial Pathologic Diagnosis Date Calculated Day Value | 0 |
| 12 | Disease Free (Months) | Range= [0, 281.29], Median=24.99 |
| 13 | Disease Free Status | categories: NA, 0: DiseaseFree, 1: Recurred/Progressed |
| 14 | Months of disease-specific survival | Range= [0, 282], Median=27.0 |
| 15 | Disease-specific Survival status | categories: NA, 0:ALIVE OR DEAD TUMOR FREE, 1:DEAD WITH TUMOR |
| 16 | Ethnicity Category | categories: NA, Not Hispanic or Latino, Hispanic or Latino |
| 17 | Form completion date | Date |
| 18 | Fraction Genome Altered | Range= [0, 1], Median=0.251 |
| 19 | Genetic Ancestry Label | categories: EUR, AFR, AFR_ADMIX, NA, EAS, SAS_ADMIX, AMR, EUR_ADMIX, SAS, ADMIX, EAS_ADMIX |
| 20 | Neoplasm Histologic Grade | NA |
| 21 | Neoadjuvant Therapy Type Administered Prior To Resection Text | categories: YES, NO, NA |
| 22 | ICD-10 Classification | categories: C50.9, C50.5, C50.2, C50.3, C50.8, C50.4 |
| 23 | International Classification of Diseases for Oncology, Third Edition ICD-O-3 Histology Code | 22 categories: 8520/3, 8500/3, 8523/3, 8200/3, 8522/3, 8507/3, 8013/3, 8401/3, 8480/3, 8575/3, 8524/3, 8010/3, 8541/3, 8022/3, 8050/3, 9020/3, 8502/3, 8510/3, 8503/3, 8201/3, 8211/3, 8090/3 |
| 24 | International Classification of Diseases for Oncology, Third Edition ICD-O-3 Site Code | categories: C50.9, C50.5, C50.2, C50.3, C50.8, C50.4 |

| | | |
|---|---|---|
| 25 | Informed consent verified | Only YES |
| 26 | In PanCan Pathway Analysis | categories: YES, NO |
| 27 | MSI MANTIS Score | Range= [0.22, 0.83], Median=0.297 |
| 28 | MSIsensor Score | Range= [0, 32.92], Median=0.19 |
| 29 | Mutation Count | Range= [1, 5400], Median=39 |
| 30 | New Neoplasm Event Post Initial Therapy Indicator | categories: YES, NO, NA |
| 31 | Oncotree Code | categories: ILC, IDC, BRCNOS, IMMC, MBC, BRCA |
| 32 | Overall Survival (Months) | Range= [0, 282], Median=27.0 |
| 33 | Overall Survival Status | categories: 0:LIVING, 1:DECEASED |
| 34 | Other Patient ID | IDs |
| 35 | American Joint Committee on Cancer Metastasis Stage Code | categories: MX, M0, M1, CM0 (I+) |
| 36 | Neoplasm Disease Lymph Node Stage American Joint Committee on Cancer Code | categories: NX, N1A, N0 (I+), N2A, N0, N0 (I-), N1, N3C, N1MI, N3A, N2, N3, N1B, N1C, N0 (MOL+), N3B |
| 37 | American Joint Committee on Cancer Tumor Stage Code | categories: TX, T2, T1C, T3, T1, T4B, T1B, T4D, T4, T1A, T2B, T3A, T2A |
| 38 | Person Neoplasm Cancer Status | categories: Tumor Free, With Tumor, NA |
| 39 | Progress Free Survival (Months) | Range= [0, 281.29], Median=25.12 |
| 40 | Progression Free Status | categories: 0:CENSORED, 1:PROGRESSION, NA |
| 41 | Primary Lymph Node Presentation Assessment | categories: YES, NO, NA |
| 42 | Prior Diagnosis | categories: YES, NO, NA |
| 43 | Race Category | categories: White, Black or African American, Asian, American Indian or Alaska Native, NA |
| 44 | Radiation Therapy | categories: YES, NO, NA |
| 45 | Ragnum Hypoxia Score | Range= [-24, 30], Median=4 |
| 46 | Number of Samples Per Patient | 1 |
| 47 | Sample Type | Primary |
| 48 | Sex | categories: Female, Male |
| 49 | Somatic Status | Matched |
| 50 | Subtype | categories: BRCA_LumA, BRCA_Her2, BRCA_LumB, BRCA_Normal, BRCA_Basal, NA |
| 51 | Tissue Prospective Collection Indicator | categories: YES, NO, NA |
| 52 | Tissue Retrospective Collection Indicator | categories: YES, NO, NA |
| 53 | Tissue Source Site | categories: Columbia University, Proteogenex, Inc., University of Sao Paulo, Holy Cross, UCSF, Walter Reed, Christiana Healthcare, Indivumed, International Genomics Consortium, Cureline, MSKCC, UNC, Mayo, Duke, University of Pittsburgh, ILSBio, Greater Poland Cancer Center, Roswell Park, Asterand, University of Miami, ABS - IUPUI, MD Anderson, Ontario Institute for Cancer Research (OICR), ABS - Research Metrics Pakistan, Hartford Hospital, Candler, Gundersen Lutheran Health System, University of Minnesota, Mount Sinai School of Medicine, University of Chicago, Fox Chase, Institute of Human Virology Nigeria, |

| | | |
|---|---|---|
| | | Albert Einstein Medical Center, Boston Medical Center, Mary Bird Perkins Cancer Center - Our Lady of the Lake, Medical College of Georgia, Greenville Health System, University of Kansas, Spectrum Health, John Wayne Cancer Center |
| 54 | Tissue Source Site Code | categories: MS, OK, OL, PE, PL, S3, UL, UU, V7, W8, WT, XX, Z7 |
| 55 | TMB (nonsynonymous) | Range= [0, 180.83], Median=1.3 |
| 56 | Tumor Disease Anatomic Site | Only Breast |
| 57 | Tumor Type | categories: Infiltrating Lobular Carcinoma, Infiltrating Ductal Carcinoma, Other, Mixed Histology (NOS), Mucinous Carcinoma, Metaplastic Carcinoma, Infiltrating Carcinoma (NOS), Medullary Carcinoma, Breast Invasive Carcinoma |
| 58 | Patient Weight | NA |
| 59 | Winter Hypoxia Score | Range= [-72, 78], Median=-14 |

*Table 2. BCNB dataset*

| | Variable | Description |
|---|---|---|
| 1 | Age(years) | Range= [23, 90], Median=57 |
| 2 | Tumour Size(cm) | Range= [0.5, 5.5], Median=2 |
| 3 | Tumour Type | Invasive ductal carcinoma, Invasive lobular carcinoma, Other type |
| 4 | ER | Positive/Negative |
| 5 | PR | Positive/Negative |
| 6 | HER2 | Positive/Negative |
| 7 | HER2 Expression | categories: 0, 1+, 2+, 3+ |
| 8 | Histological grading | categories: 1, 2, 3, NA |
| 9 | Surgical | categories: Axillary lymph node dissection, Sentinel lymph node biopsy |
| 10 | Ki67 | Range= [0.01, 0.90], Median=0.35 |
| 11 | Molecular subtype | categories: Luminal A, Luminal B, HER2+, Triple Negative |
| 12 | Number of lymph node metastases | Range= [0, 9], Median=0 |
| 13 | ALN status | categories: N0, N+(1-2), N+(>2) |

*Table 3. CPTAC-BRCA dataset*

| | Variable | Description |
|---|---|---|
| 1 | Age | Range= [30.9, 95.3], Median=61.5 |
| 2 | APOBEC Signature | categories: YES, NO, NA |
| 3 | Cancer type | Breast cancer |
| 4 | Cancer Type Detailed | Invasive breast carcinoma |

| | | |
|---|---|---|
| 5 | CD3 TILS Counts | categories: Range= [1, 80], not performed |
| 6 | CD3 TILS Status | categories: not performed, T, PT, NT |
| 7 | Chromosome INstability index CIN | Range= [0.03, 6.07], Median=1.15 |
| 8 | CIBERSORT Absolute Score | Range= [0.15, 2.06], Median=0.87 |
| 9 | ERBB2 Gene Amplified | categories: 0, 1 |
| 10 | ERBB2 Proteogenomic Status | categories: Positive, Negative |
| 11 | ERBB2 Updated Clinical Status | categories: Positive, Negative, NA |
| 12 | ER Updated Clinical Status | categories: Positive, Negative, NA |
| 13 | ESTIMATE Immune Score | Range= [-676.35, 2809.59], Median= 1228.42 |
| 14 | ESTIMATE Stromal Score | Range= [-1440.91, 1590.57], Median= 377.80 |
| 15 | ESTIMATE Tumor Purity | Range= [0.37, 0.96], Median= 0.66 |
| 16 | Ethnicity | categories: Black or African American, White, NA, Hispanic or Latino, Asian |
| 17 | Ischemia Time in Minutes | Range= [0.0, 30], Median= 10 |
| 18 | Mutation Count | Range= [11, 7909], Median= 67 |
| 19 | NMF Cluster | categories: Basal-I, HER2-I, LumA-I, LumB-I |
| 20 | NMF Cluster Membership Score | Range= [0.33, 1.0], Median= 0.72 |
| 21 | Number of non synonymous Mutations | Range= [12, 8705], Median= 72.5 |
| 22 | Oncotree code | BRCA |
| 23 | PAM50 | categories: Luminal A, Luminal B, HER2+, Basal |
| 24 | PR Clinical Status | categories: Positive, Negative, NA |
| 25 | Number of Samples Per Patient | 1 |
| 26 | Sex | categories: Female, NA |
| 27 | Stemness Score | Range= [0, 1], Median= 0.57 |
| 28 | TMB (nonsynonymous) | Range= [0.37, 264.63], Median= 2.25 |
| 29 | TMT Channel | 16 categories: 126.00, 126\|129N, 127C, 127C\|130C, 127N, 128C, 128C\|129C\|130N, 128N, 129C, 129C\|126, 129C\|128C, 129C\|130C, 129N, 130C, 130C\|127N, 130N |
| 30 | TMT Plex | Range= [1, 17], Median= 8 |
| 31 | TNBC Updated Clinical Status | categories: Positive, Negative, NA |
| 32 | TOP2A Gene Amplified | categories: 0, 1 |
| 33 | TOP2A Proteogenomic Status | categories: Positive, Negative |
| 34 | Tumor Stage | categories: NA, Stage IA, Stage IIA, Stage IIB, Stage III, Stage IIIA, Stage IIIB, Stage IIIC |
| 35 | xCell Immune Score | Range= [0.01, 0.48], Median= 0.06 |
| 36 | xCell Stromal Score | Range= [0.0, 0.36], Median= 0.01 |

*Table 4. GTEx-Breast dataset*

| | Variable | Description |
|---|---|---|
| 1 | Sex | categories: Female, Male |
| 2 | Age Bracket | categories: 20-29, 30-39, 40-49, 50-59, 60-69, 70-79 |
| 3 | Hardy Scale | categories: Slow death, Ventilator case, Fast death - violent, Intermediate death, Fast death - natural causes |
| 4 | Pathology Categories | categories: cyst, fibrosis, gynecomastoid, hyalinization, hyperplasia, mastopathy, metaplasia, necrosis, post_menopausal, sclerotic, atrophy, calcification, clean_specimens, no_abnormalities, macrophages |
| 5 | Pathology Notes | Very short notes including number of pieces, changes to breast tissue, etc. |

*Table 5. IMPRESS dataset (HER2 cohort)*

| | Variable | Description |
|---|---|---|
| 1 | Age | Range= [30.14, 76.4], Median= 56.05 |
| 2 | HER2 IHC (0-3) | categories: 1, 2, 3 |
| 3 | HER signal | Range= [6.22, 40.31], Median= 19.4 |
| 4 | CEP17 | Range= [1.5, 7.8], Median= 2.6 |
| 5 | ratio | Range= [1.23, 22.98], Median= 6.725 |
| 6 | ER (+-1/-0) | Positive/Negative |
| 7 | ER% | Range= [0.0, 100.0], Median= 0 |
| 8 | ER (1-3+) | categories: 1, 2, 3 |
| 9 | PR (+/-) | Positive/Negative |
| 10 | PR% | Range= [0.0, 100.0], Median= 0 |
| 11 | PR (1-3+) | 3 categories: 1, 2, 3 |
| 12 | histologic type | Ductal carcinoma, Lobular carcinoma |
| 13 | NG (1-3) | categories: 1, 2, 3 |
| 14 | Nuclear grade (1-3) | categories: 1, 2, 3 |
| 15 | Met-LN (no-0, yes-1) | categories: YES, NO |
| 16 | Excision (No-0, yes-1) | categories: YES, NO |
| 17 | Neoadjuvant (No-0, yes-1) | categories: YES, NO |
| 18 | Herceptin (No-0, yes-1) | categories: YES, NO |
| 19 | residual tumor (no-0, yes-1) | categories: YES, NO |
| 20 | tumor size | Range= [0.1, 7.0], Median= 0.85 |

| | | |
|---|---|---|
| 21 | pCR | categories: YES, NO |
| 22 | Response | categories: no/minimal, moderate, marked |
| 23 | RCB value | Range= [0.9, 4.14], Median= 1.39 |
| 24 | RCB category | categories: I, II, III |
| 25 | PD-L1-tumor (cutoff 1%) | Positive/Negative |
| 26 | PD-L1-stroma (cutoff 1%) | Positive/Negative |
| 27 | CD8-peritumoral (cutoff 10%) | Positive/Negative |
| 28 | CD8-intratumoral (cutoff 10%) | Positive/Negative |
| 29 | CD163-intratumoral (cutoff 10%) | Positive/Negative |

*Table 6. IMPRESS dataset (TNBC cohort)*

| | Variable | Description |
|---|---|---|
| 1 | Age | Range= [26.0, 74.0], Median= 51.05 |
| 2 | Post-NAC Grade | categories: 2,3, NA |
| 3 | Residual tumor size (cm) | Range= [0.02, 4.9], Median= 0.6 |
| 4 | ypT | categories: 2,3, NA |
| 5 | ypN | categories: 1a, 1mi, 2a, x |
| 6 | residual tumor (no-0, yes-1) | categories: YES, NO |
| 7 | pCR (no-0, yes-1) | categories: YES, NO |
| 8 | RCB value | Range= [0.79, 4.27], Median= 2.014 |
| 9 | RCB category | categories: 1, 2,3 |
| 10 | PD1 total (%) | Range= [0.0, 100.0], Median= 0 |
| 11 | PD-L1-tumor (%) | Range= [0.0, 100.0], Median= 0.25 |
| 12 | PD-L1-stroma (%) | Range= [0.0, 100.0], Median= 1 |
| 13 | CD8-intratumoral (%) | Range= [0.0, 100.0], Median= 5 |
| 14 | CD8-peritumoral (%) | Range= [0.0, 100.0], Median= 10 |
| 15 | CD163-intratumoral (%) | Range= [0.0, 100.0], Median= 30 |

*Table 7. Post-Nat-BRCA dataset*

| | Variable | Description |
|---|---|---|
| 1 | Age @ diagnosis | Range= [30, 83], Median= 49 |
| 2 | Menopausal status | categories: 0, 1:Postmenopausal, 2: Premenopausal, 3: Perimenopausal |
| 3 | Chemo-NAT | categories: YES, NO |
| 4 | AntiHER2-NAT | categories: YES, NO |
| 5 | RAD-NAT | categories: YES, NO |
| 6 | Endocrine-NAT | categories: YES, NO |
| 7 | Type of breast surgery | categories: Partial mastectomy/lumpectomy, Total mastectomy, Partial mastectomy/lumpectomy with at least one margin revised intraoperatively |
| 8 | Type of axillary LN surgery | categories: 0:Not performed, 1:Sentinel lymph node biopsy, 2:Axillary lymph node dissection, 1,2:Sentinel lymph node biopsy followed by Axillary lymph node dissection |
| 9 | Histological type (resection) | Invasive ductal carcinoma, Invasive lobular carcinoma, Invasive mammary carcinoma, Metaplastic carcinoma, Invasive tubular carcinoma, Pleomorphic (lobular), Classic (lobular) |
| 10 | Histology Grade (resection) | categories: 1, 2, 3 |
| 11 | Number of foci | categories: 1, 2, 3, Cannot be determined |
| 12 | ER (resection) | Positive/Negative |
| 13 | PR (resection) | Positive/Negative |
| 14 | HER IHC (resection) | categories: 0, 1, 2, 3 |
| 15 | HER-2 FISH | categories: 1, 2, NA |
| 16 | Residual tumor size (mm) | Range= [2.5, 144.7], Median= 30 |
| 17 | LVI | categories: YES, NO |
| 18 | DCIS/LCIS (%) | Range= [0.0, 100.0], Median= 10 |
| 19 | No of LN tested | Range= [0, 41], Median= 11 |
| 20 | LN involved | Range= [0, 13], Median= 1 |
| 21 | LN with regression | categories: YES, NO |
| 22 | Response in BC | categories: Probable or definitive response to presurgical therapy in the invasive carcinoma, Minimal response to presurgical therapy in the invasive carcinoma, No definitive response to presurgical therapy in the invasive carcinoma |
| 23 | Overall Cellularity | Range= [2, 90], Median= 25 |
| 24 | Size of Tumor Bed (mm) | Range= [4, 370], Median= 54.5 |
| 25 | Cell Annotations (Y/N) | categories: YES, NO |
